# Supplementary material for: From LLMs to LLM-based Agents for Software Engineering: A Survey of Current, Challenges and Future
Source: arXiv:2408.02479 source file (2025-04-13)
Supplement: Supplementary file 1 [file appendix.tex]

% \textcolor{red}{Cai: I think we may move these figures to the main text.}
% \subsection{Benchmarks}
% % \begin{figure}[h!]
% % \scriptsize
% %     \centering
% %     \includegraphics[scale=0.3]{benchmark2.png}
% %     \caption{Distribution of Benchmarks} 
% %     \label{fig:benchmark}
% % \end{figure}
% \begin{figure}[H]
% \scriptsize
%     \centering
%     \includegraphics[width=1\linewidth]{benchmark2_new.pdf}
%     \caption{Distribution of Benchmarks.} 
%     \label{fig:benchmark}
% \end{figure}
% \subsection{Evaluation Metrics}
% % \begin{figure}[h!]
% % \scriptsize
% %     \centering
% %     \includegraphics[scale=0.3]{metricsChart.png} 
% %     \caption{Top 10 Evaluation Metrics} 
% %     \label{fig:top10Metrics}
% % \end{figure}
% \begin{figure}[H]
% \scriptsize
%     \centering
%     \includegraphics[width=1\linewidth]{metricsChart_new.pdf}
%     \caption{Top 10 Evaluation Metrics.} 
%     \label{fig:top10Metrics}
% \end{figure}
